# Supplementary material for: Real-time modelling of the SARS-CoV-2 pandemic in England 2020-2023: a challenging data integration
Source: arXiv:2408.04178 source file (2024-08-08)
Supplement: Supplementary file 1 [file Appendix.pdf]

# Real-time modelling of the SARS-CoV-2 pandemic in England 2020-2023: a challenging data integration - Appendix

## A The transmission model of [1]

As explained in detail in [1] the initial SARS-COV-2 transmission model is based on an age-region-stratified SEEIIR structure (see Figure A.1).

Within each region, the infection dynamics are governed by a system of ordinary differential equations approximated in discrete time by the following set of first order difference equations:

$$
\begin{aligned}
S_{r,t_k,a} &= S_{r,t_{k-1},a}\left(1-\lambda_{r,t_{k-1},a}\delta t\right)\\
E^1_{r,t_k,a} &= E^1_{r,t_{k-1},a}\left(1-\frac{2\delta t}{d_L}\right)+S_{r,t_{k-1},a}\lambda_{r,t_{k-1},a}\delta t\\
E^2_{r,t_k,a} &= E^2_{r,t_{k-1},a}\left(1-\frac{2\delta t}{d_L}\right)+E^1_{r,t_{k-1},a}\frac{2\delta t}{d_L}\\
I^1_{r,t_k,a} &= I^1_{r,t_{k-1},a}\left(1-\frac{2\delta t}{d_I}\right)+E^2_{r,t_{k-1},a}\frac{2\delta t}{d_L}\\
I^2_{r,t_k,a} &= I^2_{r,t_{k-1},a}\left(1-\frac{2\delta t}{d_I}\right)+I^1_{r,t_{k-1},a}\frac{2\delta t}{d_I}
\end{aligned}
\tag{A.1}
$$

where: $S_{r,t_k,a}$, $E^l_{r,t_k,a}$, $I^l_{r,t_k,a}, l = 1, 2$ represent the time $t_k, k = 1, \ldots, K$, partitioning of the population of individuals in a region $r, r = 1, \ldots, n_r$, in age-

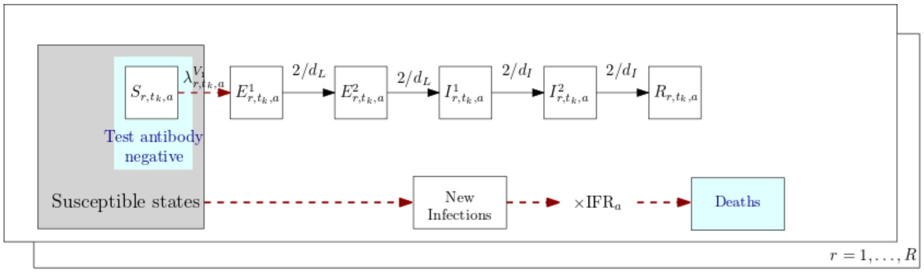


Figure A.1: Model structure as in [1]

group $a, a = 1, \dots, n_a$, into $S$ (susceptible), $E$ (exposed) and $I$ (infectious) disease states. The mean latent and infectious periods are $d_L$ and $d_I$ respectively; and $\lambda_{r,t_k,a}$ is the time- and age-varying rate with which susceptible individuals become infected. The exposed and infectious states are divided into two sub-states to approximate a continuous-time stochastic model with Erlang-distributed times in the each of these disease states. Time steps of $\delta t = 0.5$ days are chosen to be sufficiently small relative to the anticipated latent and infectious periods. New infections are generated as

$$\Delta_{r,t_k,a} = S_{r,t_k,a}\lambda_{r,t_k,a}\delta t, \tag{A.2}$$

where

$$\lambda_{r,t_k,a} = \left(1 - \prod_{a'=1}^{n_a}\left[\left(1 - b_{r,aa'}^{t_k}\right)^{I^1_{r,t_k,a'}+I^2_{r,t_k,a'}}\right]\right). \tag{A.3}$$

Here, $b_{r,aa'}^{t_k}$ is the probability of a susceptible individual in region $r$ of age group $a$ being infected by an infectious individual in age group $a'$ at time $t_k$. It is a function of:

*i.* a set of time-varying contact matrices $\boldsymbol{C}^{t_k} = \left\{C_{aa'}^{t_k}\right\}$, with $C_{aa'}^{t_k}$ describing the expected number of contacts between individuals in strata $a$ and $a'$ within a single time unit $t_k$.

*ii.* $\boldsymbol{M}_r^{t_k} = \left\{M_{r,aa'}^{t_k}\right\}$, a region-specific matrix, whose $(a,a')^{\text{th}}$ element gives the relative susceptibility of someone in age-group $a$ to an infection from an infectious individual in age-group $a'$ assuming contact between the two. Many of the components of this matrix are assumed to be 1, but some are specified as unknown parameters $m_{r,l}$, describing the relative susceptibility in the over-75s and the proportionate change in susceptibility for both under- and over-75s after the lockdown.

*iii.* $\beta_{t_k,r}$, a time-varying parameter encapsulating further temporal fluctuation in transmission that applies to all ages.

*iv.* $\mathcal{R}_{0,r}$, the initial reproduction numbers for the pandemic in each region at time $t_0$. This is a function of two free and unknown parameters, a region-specific growth rate, $\psi_r$, and $d_I$. From [2], this relationship is expressed for a SEEIIR model as:

$$\mathcal{R}_{0,r} = \psi_r d_I \frac{\left(\frac{\psi_r d_L}{2} + 1\right)^2}{1 - \frac{1}{\left(\frac{\psi_r d_I}{2}+1\right)^2}}.$$

*v.* $\mathcal{R}^*_{0,r}$, the dominant eigenvalues of the initial next-generation matrices, $\Lambda_{0,r}$:

$$\Lambda_{0,r,aa'} = N_{r,a}\tilde{C}^{t_0}_{r,aa'}d_I, \tag{A.4}$$

where $N_{r,a}$ is the population size in region $r$ and age-group $a$; and $\tilde{C}_r^{t_k}$ are a set of matrices defined by

$$\tilde{\boldsymbol{C}}_r^{t_k} = \begin{cases} \boldsymbol{M}_r^{t_{\text{lock}}-} \odot \boldsymbol{C}^{t_k} & t_k < t_{\text{lock}} \\ \boldsymbol{M}_r^{t_{\text{lock}}+} \odot \boldsymbol{C}^{t_k} & t_k \geq t_{\text{lock}} \end{cases}. \tag{A.5}$$

with the $\odot$ notation indicating element-wise multiplication, such that $A = B \odot C$ if $A_{aa'} = B_{aa'}C_{aa'}$.

The $\boldsymbol{C}^{t_k}$ matrices encode the information about contact rates between different age groups derived from the POLYMOD study [3], Google mobility and the time-use survey. The $\boldsymbol{M}_r^{t_k}$ matrices are matrices of multiplier parameters $m_{r,a}$ modifying these matrices by an age-specific susceptibility to infection given contact. These $m_{r,a}$ will be confounded with any mis-specification of the POLYMOD matrices in terms of the pattern of infection between the age groups. The $\beta_{t_k}$ parameters account for mis-specification of the changing scale of transmission over time as described by the matrices.

The general expression of $b_{r,aa'}^{t_k}$ is

$$b_{r,aa'}^{t_k} = \frac{\beta_{t_k,r}\mathcal{R}_{0,r}}{\mathcal{R}_{0,r}^*}\tilde{C}_{r,aa'}^{t_k}. \tag{A.6}$$

As this quantity varies over time, so will the reproduction number. The time-$t_k$ reproduction number is, therefore,

$$\mathcal{R}_{t_k,r} = \mathcal{R}_{0,r}\frac{\mathcal{R}_{t_k,r}^*}{\mathcal{R}_{0,r}^*} \tag{A.7}$$

where $\mathcal{R}_{t_k,r}^*$ is the dominant eigenvalue of the time $t_k$ next generation matrix, $\boldsymbol{\Lambda}_{k,r}$

$$(\Lambda_{k,r})_{aa'} = \beta_{t_k,r}S_{r,t_k,a}\tilde{C}_{r,aa'}^{t_k}d_I. \tag{A.8}$$

The transmission dynamics described above depend on the parameters $d_I$ and $d_L$ in (A.1); the parameters specifying $b_{r,aa'}^{t_k}$; and the initial conditions of the system, which can also be expressed as parameters. These unknown parameters are either fixed to values derived from the literature or estimated from the combination of different data sources linked to the latent transmission through observational models (see [1] for further details).

### Contact matrices

Time dependent contact matrices are based on location-specific POLYMOD matrices (where locations include "at work", "at home", "on transport" etc), combined with the time-use survey [4] to identify 18 different activities, including school, work, social visits, shopping etc.. The traditional POLYMOD matrices are used until 23rd March, the time of the lockdown [3, 5]. From this point on,

Table 1: The data sources used for the different activities identified by the time use survey. Values represent the assumed activity level. Where direct data was available we used other (live) data sources. Here GM represents the relevant Google mobility category.

| activity | Data source |
|---|---|
| alone | 1 |
| bars and restaurants | 0 |
| bed | 1 |
| cultural | 0 |
| exercise indoors | 0 |
| home | 1 |
| library | 0 |
| school | Attendance records |
| visit | GM Retail & recreation |
| parks | GM Parks |
| holiday | GM Retail & recreation |
| shopping | GM Retail & recreation |
| exercise outdoors | GM Retail & recreation |
| exercise unspecified | GM Retail & recreation |
| shopping essential | GM Grocery & pharmacy |
| unspecified | GM Retail & recreation |
| work | GM Workplace |
| transport | GM Transit stations |

Table 2: The fraction of contacts at home attributed to members of the household.

| AgeGroup | Contacts at home | Max contacts with household members | Fraction |
|---|---|---|---|
| $[0, 1)$ | 5.643 | 2.857 | 0.506 |
| $[1, 5)$ | 4.295 | 2.808 | 0.654 |
| $[5, 15)$ | 4.980 | 2.970 | 0.596 |
| $[15, 25)$ | 4.206 | 2.675 | 0.636 |
| $[25, 45)$ | 4.125 | 2.388 | 0.579 |
| $[45, 65)$ | 3.767 | 1.524 | 0.405 |
| $[65, 75)$ | 3.614 | 1.045 | 0.289 |
| $[75, +)$ | 3.571 | 0.714 | 0.200 |

the Google mobility and time-use survey data were used to calculate proportionate reductions in the location-specific POLYMOD matrices, which are summed together to give a weekly-varying contact matrix, $\boldsymbol{C}^{t_k} = \boldsymbol{C}^{w(t_k)} \equiv \boldsymbol{C}^{w_k}$.

Following [4] we identified 18 different activities (Table 1). Some of these activities were not allowed during lock down and, therefore, assumed to have been stopped. For other activities we used the most relevant data source. For some activities no suitable data source was available. In that case we used the retail and recreation mobility data provided by Google, because this data was assumed to best represent the general adherence level in the UK. For example, visits are unlikely to have stopped completely. Instead the retail and recreation level is used (Table 1). Note that the activities which in a well mixed model have the most effect on the base reproductive number are school, work, visits and unspecified [4].

**School attendance** School size and age range is publicly available for England. We used this to calculate the number of students for each school in the modelled age groups, based on the assumption that the students were evenly distributed across different school years. We also had access to attendance levels over time for some schools. This data was then used to calculate the average weekly attendance level in each local authority, weighted by the size of the school in that age group. Finally, we combined these values to calculate attendance in England, weighted by local authority population size. Not all schools reported attendance every week, as a result the attendance by local authority was, in rare cases, only based on the report of 1 or more small schools. To ensure that these did not skew our results, we ignored any attendance estimate based on schools with less than 100 students in total.

**Visits at home** [4] used the time usage data for visits at home to estimate the number of visit related contacts at home. We found that this underestimates the number of visitors and instead used the POLYMOD data on household size to

estimate the fraction of contacts at home with other household members versus the contacts with others (e.g. visitors). First, we extracted the mean number of contacts at home (Table 2). Next, we limited numbers of contacts at home ($c_i$) to household size ($h_i$) minus one ($\hat{c_i} = \min(h_i - 1, c_i)$), i.e. the maximum number of contacts any participant ($i$) can have with just household members and calculated the mean contacts based on that value. Note that this provides a conservative estimate of the fraction of contacts from visits, because some participants will not have met all their household members during the day.

**Google mobility data** During the pandemic Google provided aggregated mobility data from Android phones for many countries[1]. The mobility data gives an indication of the activity level for 5 different activities: retail and recreation, grocery and pharmacy, parks, transit stations, workplaces and residential. The UK data was further subdivided into activity by local authority, by matching the Google provided locations to local authority districts in England. This data was then combined, weighted by population size. Finally, the daily values were averaged by week, to produce weekly activity levels.

# B Model Dynamics

Here we give the full dynamic system of equations for the model presented in Figure 1(C). All state occupancy values below are region-dependent, but, for presentation, dependence on region $r$ is suppressed. For brevity we use the index $k$ in place of $t_k$:

[1]Available from https://www.google.com/covid19/mobility/

$$
\begin{aligned}
S^{V_q}_{k+1,a} &= S^{V_{q-1}}_{k,a} v^{q}_{k,a}\delta t + S^{V_q}_{k,a}\left(1 - v^{q+1}_{k,a}\delta_t\right)\left(1 - \left(1 - \pi^{q}_{k}\right)\lambda_{k,a}\delta t\right)\\
E^{V_q,1}_{k+1,a} &= E^{V_{q-1},1}_{k,a} v^{q}_{k,a}\delta t + \left(S^{V_q}_{k,a} + W^{V_q,S}_{k,a}\right)\left(1 - v^{q+1}_{k,a}\delta_t\right)\left(1 - \pi^{q}_{k}\right)\lambda_{k,a}\delta t\\
&\qquad + E^{V_q,1}_{k,a}\left(1 - v^{q+1}_{k,a}\delta_t\right)\left(1 - \frac{2}{d_L}\delta t\right)\\
E^{V_q,2}_{k+1,a} &= E^{V_{q-1},2}_{k,a} v^{q}_{k,a}\delta t + E^{V_q,1}_{k,a}\left(1 - v^{q+1}_{k,a}\delta_t\right)\frac{2}{d_L}\delta t + E^{V_q,2}_{k,a}\left(1 - v^{q+1}_{k,a}\delta_t\right)\left(1 - \frac{2}{d_L}\delta t\right)\\
I^{V_q,1}_{k+1,a} &= I^{V_{q-1},1}_{k,a} v^{q}_{k,a}\delta t + E^{V_q,2}_{k,a}\left(1 - v^{q+1}_{k,a}\delta_t\right)\frac{2}{d_L}\delta t + I^{V_q,1}_{k,a}\left(1 - v^{q+1}_{k,a}\delta_t\right)\left(1 - \frac{2}{d_I}\delta t\right)\\
I^{V_q,2}_{k+1,a} &= I^{V_{q-1},2}_{k,a} v^{q}_{k,a}\delta t + I^{V_q,1}_{k,a}\left(1 - v^{q+1}_{k,a}\delta_t\right)\frac{2}{d_I}\delta t + I^{V_q,2}_{k,a}\left(1 - v^{q+1}_{k,a}\delta_t\right)\left(1 - \frac{2}{d_I}\delta t\right)\\
R^{V_q,+}_{k+1,a} &= R^{V_{q-1},+}_{k,a} v^{q}_{k,a}\delta t + I^{V_q,2}_{k,a}\left(1 - v^{q+1}_{k,a}\delta_t\right)\frac{2}{d_I}\delta t + R^{V_q,+}_{k,a}\left(1 - v^{q+1}_{k,a}\delta_t\right)\left(1 - \frac{1}{d_R}\delta t\right)\\
R^{V_q,-}_{k+1,a} &= R^{V_{q-1},-}_{k,a} v^{q}_{k,a}\delta t + R^{V_q,+}_{k,a}\left(1 - v^{q+1}_{k,a}\delta_t\right)\frac{1}{d_R}\delta t + R^{V_q,-}_{k,a}\left(1 - v^{q+1}_{k,a}\delta_t\right)\left(1 - \frac{2}{d_{W,t}}\delta t\right)\\
W^{V_q,}_{k+1,a} &= W^{V_{q-1},}_{k,a} v^{q}_{k,a}\delta t + R^{V_q,-}_{k,a}\left(1 - v^{q+1}_{k,a}\delta_t\right)\frac{2}{d_{W,t}}\delta t + W^{V_q,}_{k,a}\left(1 - v^{q+1}_{k,a}\delta_t\right)\left(1 - \frac{2}{d_{W,t}}\delta t\right)\\
W^{V_q,S}_{k+1,a} &= W^{V_{q-1},S}_{k,a} v^{q}_{k,a}\delta t + W^{V_q,}_{k,a}\left(1 - v^{q+1}_{k,a}\delta t\right)\frac{2}{d_{W,t}}\delta t\\
&\qquad + W^{V_q,S}_{k,a}\left(1 - v^{q+1}_{k,a}\delta t\right)\left(1 - \left(1 - \pi^{q}_{k}\right)\lambda_{k,a}\delta t\right)
\end{aligned}
\tag{B.1}
$$

where $v^0_{k,a} = v^4_{k,a} = \pi^0_k = 0$.

# C Prevalence Estimates

Data from the Office of National Statistics (ONS) Coronavirus Infection Survey (CIS) were held on the Secure Research Service (SRS) (https://www.ons.gov.uk/aboutus/whatwedo/statistics/requestingstatistics/secureresearchservice). The SRS is a Trusted Research Environment, designed to ensure safe use of the data and, in particular, to prevent informative disclosure of information on the survey's participants. Consequently, the raw data on test results could not be extracted from the SRS for use external to the ONS. However, within the SRS these data could be used to generate estimates of RT-PCR-positive infection prevalence.

These estimates were generated in a multi-level regression with poststratification (MRP) process. Here, the MRP was applied within each region independently of the other regions in two distinct stages. In the first stage the number of people testing positive on day $t$ in age-group $a$ in region $r$, $x_{rta}$, was assumed to be a realisation of a beta-binomially distributed random variable (the data were assumed to be over-dispersed due to the household structure of the survey). If $n_{rta}$ tests were conducted:

$$X_{rta} \sim \text{Beta-Binomial}\left(n_{rta}; p_{rta}, \rho_r\right)$$

such that $\mathbb{E}X_{rta} = n_{rta}p_{rta}$ and $\text{Var}(X_{rta}) = n_{rta}p_{rta}(1-p_{rta})(1+(n_{rta}-1)\rho_r)$, with hyperparameter $0 < \rho_r < 1$ being such that independent and identically distributed $\text{logit}(\rho_r) \sim \text{N}(0, 2.5)$.

A two-level Gaussian Markov Random Field model is specified for the positivity in each region:

$$\text{logit}\,(p_{rta}) = u_{ra} + v_{rt} + w_{rta}$$

where

- $u_{ra}$ are iid random effects, $u_{ra} \sim \text{N}(0, \sigma_r^2)$. The hyperparameters $\sigma_r$ have a penalised complexity prior such that $\mathbb{P}(\sigma_r > 1) = 0.1$, with the corresponding density defined on the precision, $\tau_r = \sigma_r^{-2}$:

  $$\pi\,(\tau_r) = \frac{\lambda}{2}\tau_r^{-3/2}\exp\left(-\lambda\tau_r^{-1/2}\right), \tau_r > 0$$

  where $\lambda = -\log(0.1)$.

- $v_{rt}$ is a population level second-order random-walk, such that $v_{rt} = 2v_{r,t-1} - v_{r,t-2} + \epsilon^v_{rt}$, where $\epsilon^v_{rt} \sim \text{N}(0, e^{-\theta^v_r})$, with independent and identically distributed $\theta^v_r \sim \Gamma(1, 5e^{-5})$.

- $w_{rta}$ are age-specific, independent, second-order random-walks, $w_{rta} = 2w_{r,t-1,a} - w_{r,t-2,a} + \epsilon^w_{rt}$, where $\epsilon^w_{rt} \sim \text{N}(0, e^{-\theta^w_r})$, $\theta^w_r \sim \Gamma(1, 5e^{-5})$.

This model was implemented using the integrated nested Laplace approximation (INLA, [6]), to obtain posterior summaries for the $p_{rta}$ in terms of the mean ($\tilde{p}_{rta}$) and standard deviation ($\text{sd}(p_{rta})$). These are then scaled by ONS estimates for the number of people in each region and age-group at all times, to give a posterior mean number of people who would test PCR positive for each region/age/time combination, $\tilde{Z}_{rta}$ and corresponding posterior standard deviation $\tilde{\xi}_{rta}$, and it is these values that are extracted from the ONS TRE.

# D Adaptive Metropolis with Global Scaling (AMGS) algorithm

With the rapidly expanding dimension of the parameter space and the requirement to provide pandemic insights in a timely manner, engineering an MCMC algorithm that could achieve convergence and sample from the desired posterior distributions was a significant challenge.

The algorithm that was eventually settled upon is a variation of an algorithm introduced by [7] and detailed in [8]. Here, we outline the algorithm and highlight any adaptations made.

## D.1 A general updating scheme

As discussed in Section 2.3.2, the models can be partitioned according to whether they are region-specific ('regional') or apply to all regions ('global'). This partitioning of the dimensions of the parameter vector can be exploited as it is possible to update regional parameters in parallel, in blocks corresponding to each region. Therefore, consider a partitioning of the parameter vector $\boldsymbol{\theta} = (\boldsymbol{\theta}^{\mathrm{r}}_1, \ldots, \boldsymbol{\theta}^{\mathrm{r}}_R, \boldsymbol{\theta}^{\mathrm{g}})$, where the $\boldsymbol{\theta}^{\mathrm{r}}_r, r = 1, \ldots, R$ are region-specific blocks that are updated in parallel, and $\boldsymbol{\theta}^{\mathrm{g}}$ is a single block of global parameters updated serially. Denote $\mathcal{D}_{r,t_k}$ to represent the totality of data observed in region $r$ up to time $t_k$:

To derive a sample at time $t_k$, the general algorithm will proceed

**Algorithm 1** MCMC that targets the posterior of interest.

Set the number of iterations $\nu$.
**for** $i = 1, \ldots, \nu$ **do**
  **for** $r = 1, \ldots, R$ **do**
    Draw $\boldsymbol{\theta}^{\mathrm{r}}$ from $p(\boldsymbol{\theta}^{\mathrm{r}}|\boldsymbol{\theta}^{\mathrm{g}}, \mathcal{D}_{r,t_k})$   } in parallel.
  **end for**
  Draw $\boldsymbol{\theta}^{\mathrm{g}}$ from $p(\boldsymbol{\theta}^{\mathrm{g}}|\boldsymbol{\theta}^{\mathrm{r}}_{1:R}, \mathcal{D}_{r,t_k})$.
**end for**

## D.2 Adaptive Metropolis with Global Scaling (AMGS)

In total, there will be $M = R + 1$ parameter blocks. The MCMC proceeds by using the AMGS algorithm (see [7]) to update the parameters within each block. For any generic block, denoted $\boldsymbol{\theta}_m$, the algorithm requires that we learn a covariance matrix $\boldsymbol{\Sigma}_m$ for the proposal distribution.

The algorithm is comprehensively detailed in [8], here only a brief overview is provided. If we denote $\boldsymbol{\theta}^i_m$ to be the $m^{\mathrm{th}}$ parameter block at the $i^{\mathrm{th}}$ iteration:

*i.* **Propose** $\boldsymbol{\theta}^*_m \sim N(\boldsymbol{\theta}^i_m, \lambda^i_m \Sigma^i_m)$. Set $\boldsymbol{\theta}^{i+1}_m = \boldsymbol{\theta}^*_m$ with the standard Metropolis-Hastings acceptance probability (see, for example, [9]), denoted $\alpha(\boldsymbol{\theta}^i_m, \boldsymbol{\theta}^*_m)$. Else set $\boldsymbol{\theta}^{i+1}_m = \boldsymbol{\theta}^i_m$.

*ii.* **Iterate** If $i > i_0$, for some small number of initial iterations, taken here to be $i_0 = 200$, update $\lambda^i_m$ and $\Sigma^i_m$ using recursions:

- $\mu^{i+1}_m = \mu^i_m + \gamma^{i+1}(\boldsymbol{\theta}^{i+1}_m - \mu^i_m)$
- $\Sigma^{i+1}_m = \Sigma^i_m + \gamma^{i+1}[(\boldsymbol{\theta}^{i+1}_m - \mu^i_m)(\boldsymbol{\theta}^{i+1}_m - \mu^i_m)^\top - \Sigma^i_m]$
- $\log(\lambda^{i+1}_m) = \log(\lambda^i_m) + \gamma^{i+1}[\alpha(\boldsymbol{\theta}^i_m, \boldsymbol{\theta}^{i+1}_m) - \alpha^\star]$, for some optimal $\alpha^\star$ representing a desired acceptance rate. From [10], $\alpha^* = 0.234$.
- $\gamma^i = (i - 199)^{-0.6}$. This ensures that the adaptation gets vanishingly small as $i$ gets large, a necessary condition for the ergodicity of the Markov chain.

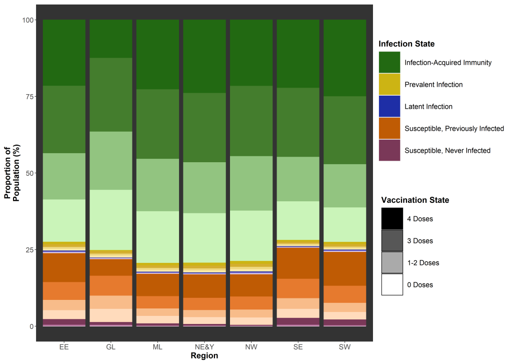


Figure E.1: Proportion of the population by infection status (susceptible, latent infection, infectious, infection-acquired immunity) and number of vaccine doses, stratified by region. For further description see Figure 2(A) and supporting text.

### D.3 Customising AMGS

The algorithm of section D.2 began to perform poorly around November 2021. The proposal parameters for each parameter block are continually adapted throughout the MCMC. It was felt that this might lead to over-adaptation. Instead we used early-stopping regularisation, as proposed by [11]. This involved specifying

- a fixed adaptation period, of $i_A$ iterations
- a range of acceptable acceptance probabilities $(\alpha^*_-, \alpha^*_+)$
- an adaptation interval, $\Delta i$.

Adaptation, as specified by in $ii$ above, will then take place only if $i < i_A$, if $i$ is a multiple of $\Delta i$ iterations, and if $\hat{S}_{\lambda_m,\Sigma_m}$, the mean acceptance ratio over the previous $\Delta i$ iterations lies outside the interval $(\alpha^*_-, \alpha^*_+)$. Similarly, sample means and covariances over the previous $\Delta i$ iterations are used in the expressions for $\mu_m^{i+1}$ and $\Sigma_m^{i+1}$ respectively.

## E Additional results and Goodness-of-fit

### E.1 Sensitivity to choice of dataset

To illustrate how sensitive our results are to the precise choice of time series data, the estimated incidence curves in Figure E.5 in blue and green are both based on the data on deaths, with the green curve using the full time series whereas the blue curve is estimated without using the death data beyond 1st April 2022. The lack of difference between these two curves suggests that, given the prevalence

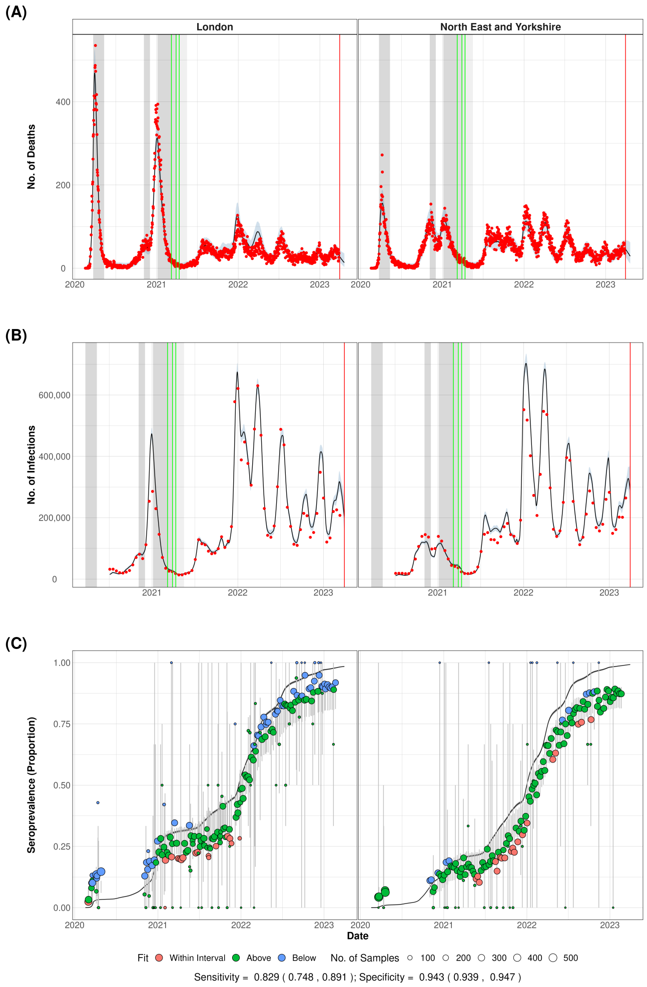


Figure E.2: Goodness-of-fit plots equivalent to figure 5 for regions London and the North East.

and serology data, the data on deaths are not overly influential (though they do permit an estimate of the infection-fatality ratio). The red curve, based on admissions, does differ, with a very different epidemic trend being projected over the last six weeks of the analysis. This trend appears more uncertain at the analysis time due to $R_t$ being close to 1 (though this uncertainty is much reduced in the results aggregated to the national level). The estimation based on deaths, however, shows a continued decline. Historically, the two estimated epidemic curves are more similar, with the admissions-based curve being slightly smoother around peaks and there being a slight phase difference throughout.

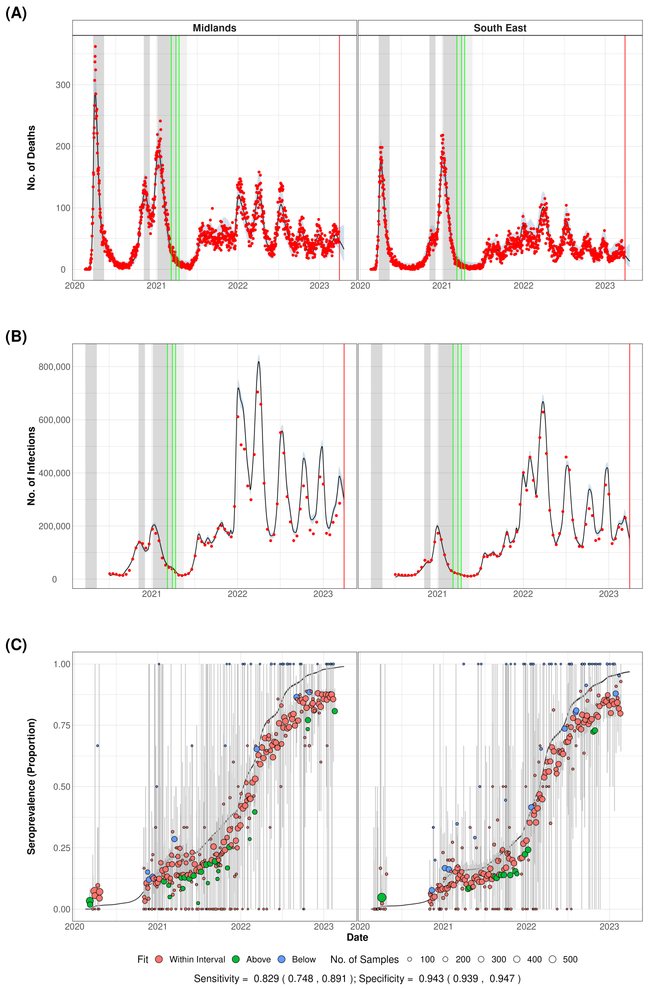


Figure E.3: Goodness-of-fit plots equivalent to figure 5 for regions Midlands and the South East.

With the concerns around the changes to testing policy, it is preferred to base modelling only on the testing of new admissions to hospital, as these are more likely to represent incidence of severe infections.

# References

[1] P. Birrell, J. Blake, E. van Leeuwen, N. Gent, D. De Angelis, *Philosophical Transactions of the Royal Society B* **376** (2021).

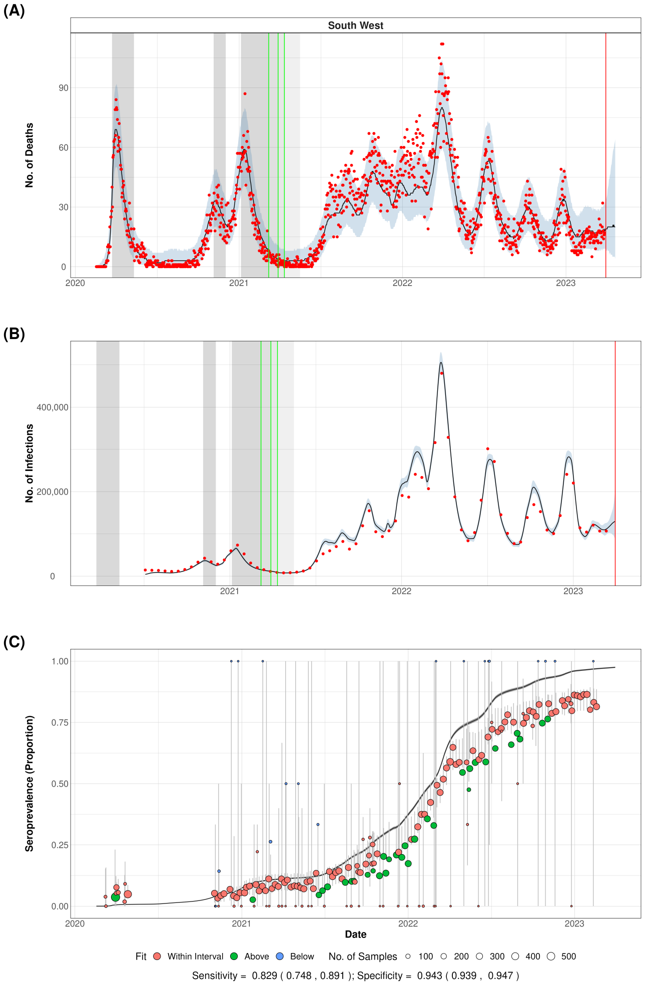


Figure E.4: Goodness-of-fit plots equivalent to figure 5 for the South West.

[2] H. J. Wearing, P. Rohani, M. J. Keeling, *PLOS Medicine* **2**, e174 (2005).

[3] J. Mossong, *et al.*, *PLoS medicine* **5**, e74 (2008).

[4] E. van Leeuwen, {PHE Joint modelling group}, F. Sandmann, *Statistical Methods in Medical Research* **31**, 1704 (2022).

[5] S. Funk, socialmixr: Social mixing matrices for infectious disease modelling, The Comprehensive R Archive Network, `http://datacompass.lshtm.ac.uk/646/` (2018).

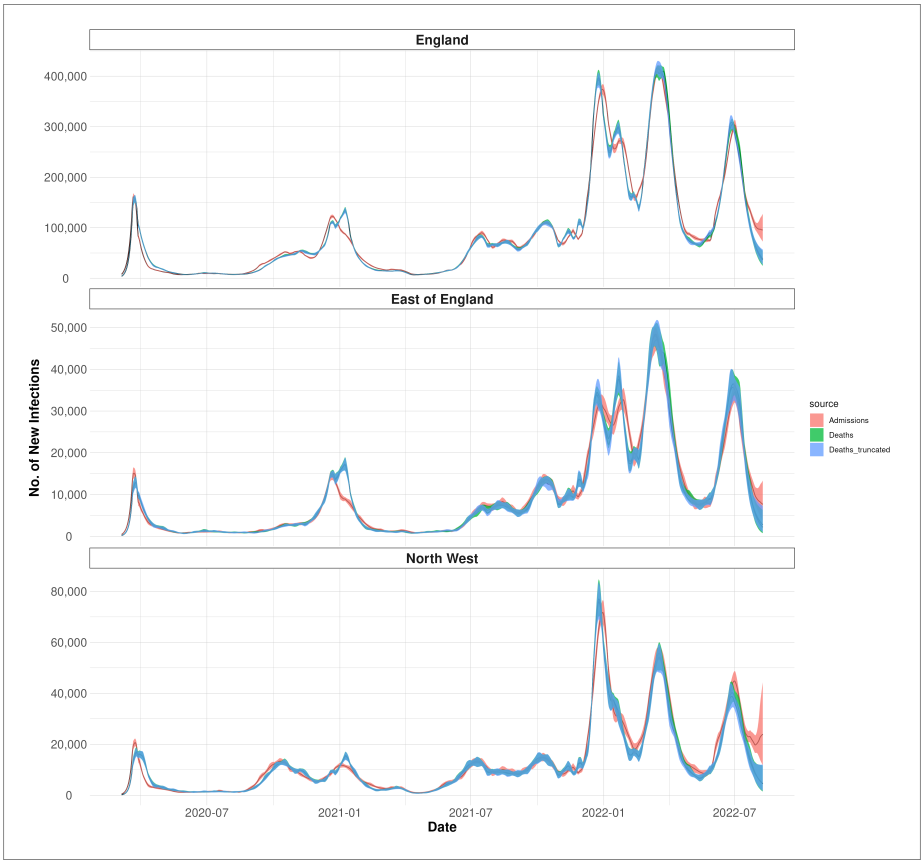


Figure E.5: Smoothed estimates (using a 7-day rolling average) of the number of new daily infections in England, the East of England and the North West using data on: daily diagnoses in new hospital admissions (red); daily deaths within 28 days of a positive test (green); and the same deaths dataset truncated on the 1$^{st}$ April, 2022 (blue).

[6] H. Rue, S. Martino, N. Chopin, *Journal of the Royal Statistical Society Series B* **71**, 319 (2009).

[7] C. Andrieu, J. Thoms, *Statistics and Computing* **18**, 343 (2008).

[8] S. Ghosh, P. J. Birrell, D. D. Angelis, *PLOS Computational Biology* **19**, e1011088 (2023).

[9] S. P. Brooks, *Journal of the Royal Statistical Society: Series D (The Statistician)* **47**, 69 (1998).

[10] G. O. Roberts, J. S. Rosenthal, *Statistical Science* **16**, 351 (2001).

[11] T. Zhang, B. Yu, *Annals of Statistics* **33**, 1538 (2005).
